# Supplementary material for: Tunable Enhancement of Magnetization Dynamics by Crystal Cut at Interface Exchange Coupled $\alpha$-Fe$_2$O$_3$/NiFe Heterostructures
Source: arXiv:2412.14090 ancillary file (2025-04-08)
Supplement: Supplementary file 1 [file Hematite-Py_SI.pdf]

# Néel-vector Control of Magnetization Dynamics in $\alpha$ -Fe<sub>2</sub>O<sub>3</sub>/NiFe Heterostructures

Hassan Al-Hamdo,<sup>1,\*</sup> Tobias Wagner,<sup>2,†</sup> Philipp Schwenke,<sup>1</sup> Gutenberg  
Kendzo,<sup>1</sup> Maximilian Dausend,<sup>1</sup> Laura Scheuer,<sup>1</sup> Misbah Yaqoob,<sup>1</sup> Vitaliy  
I. Vasyuchka,<sup>1</sup> Philipp Pirro,<sup>1</sup> Olena Gomonay,<sup>2</sup> and Mathias Weiler<sup>1</sup>

<sup>1</sup>*Fachbereich Physik and Landesforschungszentrum OPTIMAS,*

*Rheinland-Pfälzische Technische Universität*

*Kaiserslautern-Landau, 67663 Kaiserslautern, Germany*

<sup>2</sup>*Institute of Physics, Johannes Gutenberg-University Mainz, 55099 Mainz, Germany*

## **( $\alpha$ -Fe<sub>2</sub>O<sub>3</sub>): CRYSTALLOGRAPHY AND MAGNETIC PROPERTIES**

$\alpha$ -Fe<sub>2</sub>O<sub>3</sub>, chemically denoted as  $\alpha$ -Fe<sub>2</sub>O<sub>3</sub>, is a ubiquitous iron oxide mineral and represents one of the main sources of iron. It is found extensively in the sedimentary rocks of Earth's crust and is the end product of the weathering of iron-bearing minerals. The hexagonal crystal structure of  $\alpha$ -Fe<sub>2</sub>O<sub>3</sub> falls under the space group R-3c, with lattice parameters  $a = 5.067 \text{ \AA}$  and  $c = 13.882 \text{ \AA}$  [1]. This mineral's inherent electrical insulation properties couple with intriguing magnetic behaviors, making it a focal point in magnetism research.

The transition of  $\alpha$ -Fe<sub>2</sub>O<sub>3</sub> from a paramagnetic to an antiferromagnetic state at its Néel temperature ( $T_N$ ) of approximately 950 K underscores its complex thermal magnetic behavior [2]. The Morin transition at about 260 K, where  $\alpha$ -Fe<sub>2</sub>O<sub>3</sub> undergoes a change in its magnetic properties, is of particular importance [3, 4]. This transition has been the subject of extensive study due to its implications in both geological and material sciences.

### **Magnetic Phases of $\alpha$ -Fe<sub>2</sub>O<sub>3</sub>**

$\alpha$ -Fe<sub>2</sub>O<sub>3</sub> exhibits two primary magnetic phases influenced by the Morin transition temperature ( $T_M$ ):

1. **Weak Ferromagnetism (WFM):** Above ( $T_M$ ), weak ferromagnetism occurs in  $\alpha$ -Fe<sub>2</sub>O<sub>3</sub>. This condition arises from the slight canting of spins, away from their antiparallel alignment, influenced by the Dzyaloshinskii–Moriya interaction. This magnetic phase is characterized by the generation of a weak magnetic moment, which reverts to collinear antiferromagnetism as temperatures decline to  $T_M$ .
2. **Collinear Antiferromagnetism:** Below  $T_M$ , the magnetic structure of  $\alpha$ -Fe<sub>2</sub>O<sub>3</sub> is predominantly collinear antiferromagnetic. In this phase, iron ions' magnetic moments are perfectly antiparallel, effectively canceling each other out and thus producing no net macroscopic magnetization.

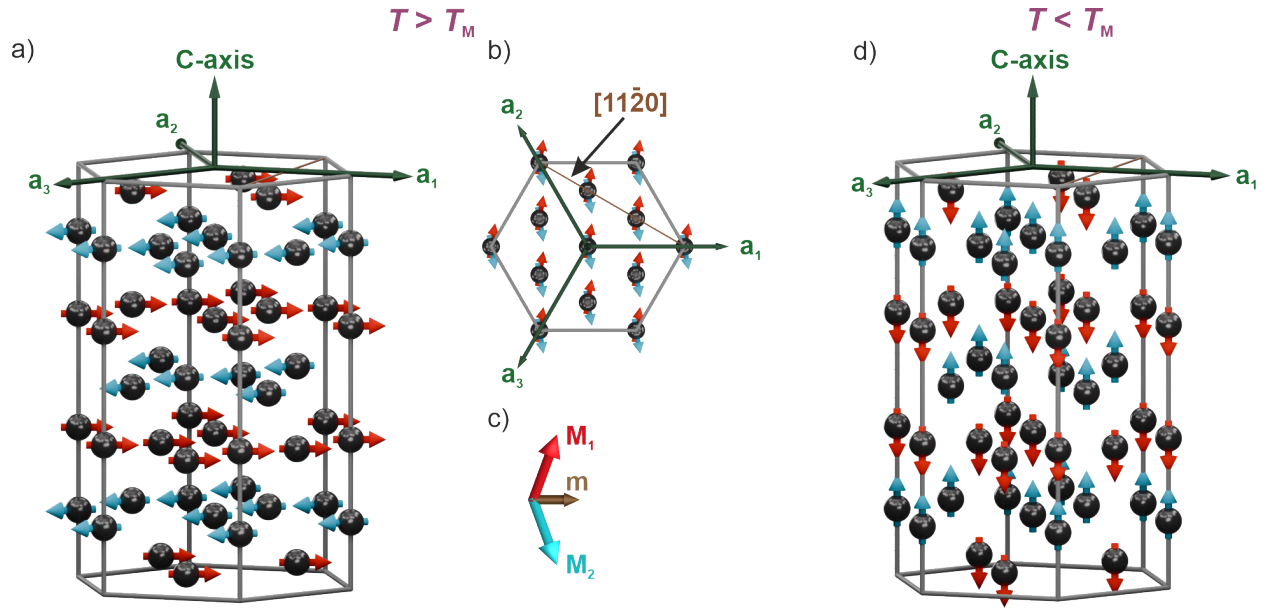

FIG. S1. Hexagonal unit cell of crystal structure of  $\alpha\text{-Fe}_2\text{O}_3$  in different magnetic states. Panel (a) and (b) depict the high-temperature phase with canted antiferromagnetism, while panels (c) and (d) illustrate the low-temperature collinear antiferromagnetic state.

## SAMPLES AND FABRICATION PROCESS

In this study, we employed commercially acquired natural bulk  $\alpha$ -Fe<sub>2</sub>O<sub>3</sub> crystals from SurfaceNet GmbH, each with dimensions of  $10 \times 10 \times 1$  mm. These samples were precisely cut to explore different basal plane orientations, specifically  $(11\bar{2}0)$ ,  $(0001)$ ,  $(10\bar{1}0)$ , and  $(1\bar{1}02)$ , each with two unique in-plane orientations to facilitate comprehensive analysis:

- The  $(11\bar{2}0)$  orientation with in-plane orientations  $[0001]$  and  $[1\bar{1}00]$ .
- The  $(0001)$  orientation with in-plane orientations  $[1\bar{1}02]$  and  $[1\bar{1}00]$ .
- The  $(10\bar{1}0)$  orientation with in-plane orientations  $[0001]$  and  $[1\bar{2}10]$ .
- The  $(1\bar{1}02)$  orientation with in-plane orientations  $[1\bar{1}02]$  and a projection on  $[1\bar{1}00]$ .

Both sides of each sample were meticulously polished to ensure a deformation-free and perfectly smooth surface.

Figure S2 presents the unit cell of  $\alpha$ -Fe<sub>2</sub>O<sub>3</sub> along with the main planes of our samples. This selection is aimed at covering all significant planes within the hexagonal structure to study the influence of crystal orientation on the magnetic properties of  $\alpha$ -Fe<sub>2</sub>O<sub>3</sub> at 300 Kelvin and to examine the dependence of interfacial exchange coupling in  $\alpha$ -Fe<sub>2</sub>O<sub>3</sub>/Py heterostructures with varying main and in-plane orientations.

For the investigation of interfacial exchange coupling, a Py layer was deposited onto the  $\alpha$ -Fe<sub>2</sub>O<sub>3</sub> at room temperature. This deposition process was conducted using molecular beam epitaxy (MBE) under ultra-high vacuum conditions at  $10^{-11}$  mbar. Prior to deposition, the sample surfaces were cleaned via plasma etching, which involved heating the samples up to 200°C to remove any surface contaminants. Following etching, the samples were transferred in vacuum to the deposition chamber. The Py deposition was carried out at a rate of 1 Å/s. Finally, an Al<sub>2</sub>O<sub>3</sub> capping layer of 3 nm thickness was applied to protect the Py layer from oxidation.

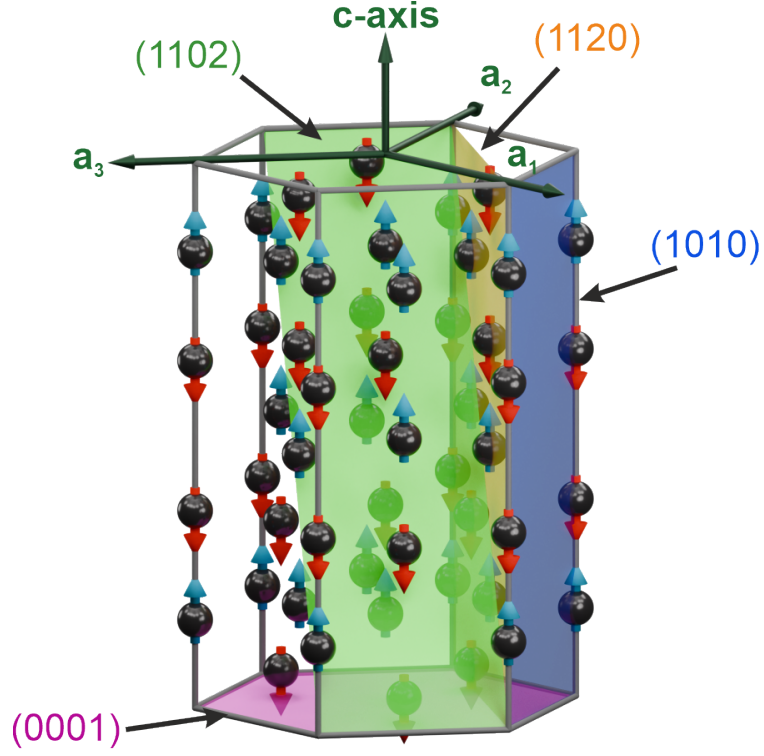

FIG. S2. Crystal cuts of  $\alpha$ -Fe<sub>2</sub>O<sub>3</sub> depicted in the hexagonal coordinate system  $\vec{a}_1$ ,  $\vec{a}_2$ ,  $\vec{a}_3$ ,  $\vec{c}$ . The two magnetic sublattices of  $\alpha$ -Fe<sub>2</sub>O<sub>3</sub> are shown in red and blue. For detailed information on the orientation of the indicated crystal cuts, please refer to Tab. S2.

## LOW TEMPERATURE FMR MEASUREMENTS

To investigate the spin dynamics of our samples, we performed Vector Network Analyzer Ferromagnetic Resonance (VNA-FMR) measurements using Cryogenic Ferromagnetic Resonance Spectroscopy (Cryo-FMR) in frequency sweep mode, across a temperature range from 40 K to room temperature. During these measurements, we recorded the complex microwave transmission parameter  $S_{21}$ , with the RF signal generated at port 1 and detected at port 2 of the VNA. The VNA was connected to a coplanar waveguide (CPW) via microwave cables and end-launch connectors, with the CPW mounted within an electromagnet.

The experiments were conducted in an in-plane configuration using a Rohde & Schwarz ZNB43 Vector Network Analyzer with a frequency range up to 43.5 GHz. The RF signal was delivered to the sample through a straight CPW with an 75  $\mu\text{m}$ -wide center conductor. All measurements were performed at a consistent RF power level of -10 dBm. By analyzing the phase and amplitude of the microwave transmission parameter  $S_{21}$ , we determined the absorption of RF power by the sample as a function of frequency. An external magnetic field up to 0.5 T was applied in-plane to the samples. Measurements were taken along two different orientations by rotating the field by 90° to align with another in-plane orientation of the sample. The magnetic field values were monitored using a Hall probe placed directly above the sample. The field was varied between 0 and 0.5 T in increments of 4.5 mT. At each field step, frequencies from 1 to 40 GHz were scanned with a resolution of 20 MHz, capturing the real and imaginary components of the complex microwave transmission parameter  $S_{21}$  as a function of the external magnetic field. To ensure measurement accuracy, the field values were recorded both before and after each frequency sweep. To remove frequency-dependent background noise from our VNA-FMR measurements, we calculated the normalized field derivative  $d_D S_{21}$ , following the methodology described in the literature [5].

The FMR spectra of the samples were measured before Py deposition using a rotatable electromagnet to assess the in-plane anisotropy of each sample, as illustrated in Fig. S3. The results indicate that the samples exhibit varying degrees of in-plane anisotropy.

Fig.S3 presents the background-corrected, frequency-dependent  $\text{Re}(d_D S_{21}/dH)$  VNA-FMR data obtained from all samples without Py. Measurements were conducted for each sample with a fixed external magnetic field of  $\mu_0 H_0 = 0.2 \text{ T}$  at room temperature. The data reveal a noticeable variation in the  $\alpha\text{-Fe}_2\text{O}_3$  signal, indicating an in-plane anisotropic

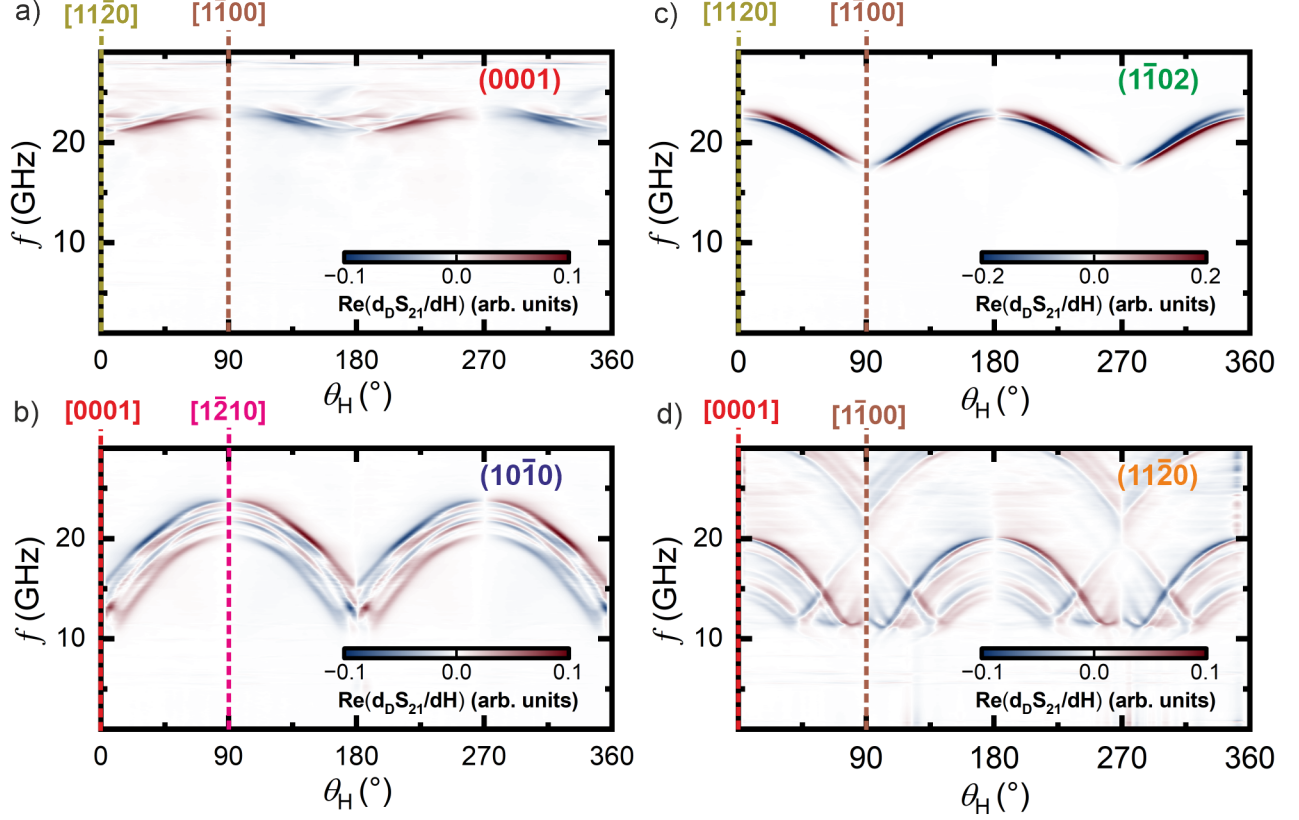

FIG. S3. The real part of the angle-dependent spectra for all samples, prior to depositing a Py layer, was obtained with a fixed applied external magnetic field of  $\mu_0 H_0 = 0.2$  T at 300 K.

behavior with a periodicity of 90 degrees. This anisotropic behavior is also influenced by the crystal orientation of the sample. For instance, while the frequency shift for the (0001) sample is around 3 GHz, it is approximately 10 GHz for the (10 $\bar{1}$ 0) sample. Notably, the easy axis for the magnetic moment of  $\alpha$ -Fe<sub>2</sub>O<sub>3</sub> along the [0001] direction in the (10 $\bar{1}$ 0) sample is the hard axis for the Néel vector, as the angle between them is approximately 83° [2].

To study temperature-dependence spin dynamics in  $\alpha$ -Fe<sub>2</sub>O<sub>3</sub>/Py stacks. The system was initially cooled to 35 K, and the temperature near the sample was monitored by a sensor positioned directly underneath. A heater located beneath the sample holder was used to reach the desired temperatures. Once the target temperature was achieved, the system was allowed to stabilize for approximately 15 min to ensure thermal equilibrium across the sample. Measurements were conducted under vacuum conditions at a pressure of  $10^{-7}$  mbar. Temperature sweeps were initiated from 40 K to 250 K in 10 K increments. For the range between 250 K and 258 K, finer steps of 1 K were utilized. In the critical range from 259 K

to 262 K, the temperature increments were further reduced to 0.5 K for more detailed data acquisition. Beyond 270 K, measurements continued with 10 K increments up to 400 K.

Figure S4 presents a schematic of the  $(10\bar{1}0)$  sample stack with the external magnetic field  $H_0$  aligned along the in-plane crystallographic orientations  $[0001]$  and  $[1\bar{2}10]$ . When  $H_0$  is aligned along  $[0001]$ , the ferromagnetic resonance (FMR) spectra of  $\alpha\text{-Fe}_2\text{O}_3$  at 300 K, as shown in Figure S4(b), exhibit two distinct resonance modes. The first resonance mode appears at 8 GHz when  $H_0 = 0$  T and increases in frequency as the external magnetic field strength increases. The second resonance mode occurs at frequencies ranging from 11 to 13 GHz at zero field and also shows a slight upward trend with increasing external field strength. Notably, in this orientation, the resonance signal from the Py layer is weak and does not exhibit any enhancement. According to our model, at 300 K, the Néel vector  $\mathbf{n}$  and the magnetization vector  $\mathbf{m}_F$  are perpendicular to each other. This perpendicular alignment results in the absence of interfacial exchange coupling between the layers.

However, upon cooling the system to 40 K (Fig. S4 (c)), the Py signal exhibits a significant enhancement, with the frequency increasing up to 7 GHz at  $\mu_0 H_0 = 0$  T. . At this lower temperature, both  $\mathbf{n}$  and  $\mathbf{m}_F$  become parallel, leading to coupling between the spin systems of both layers, as predicted by our model.

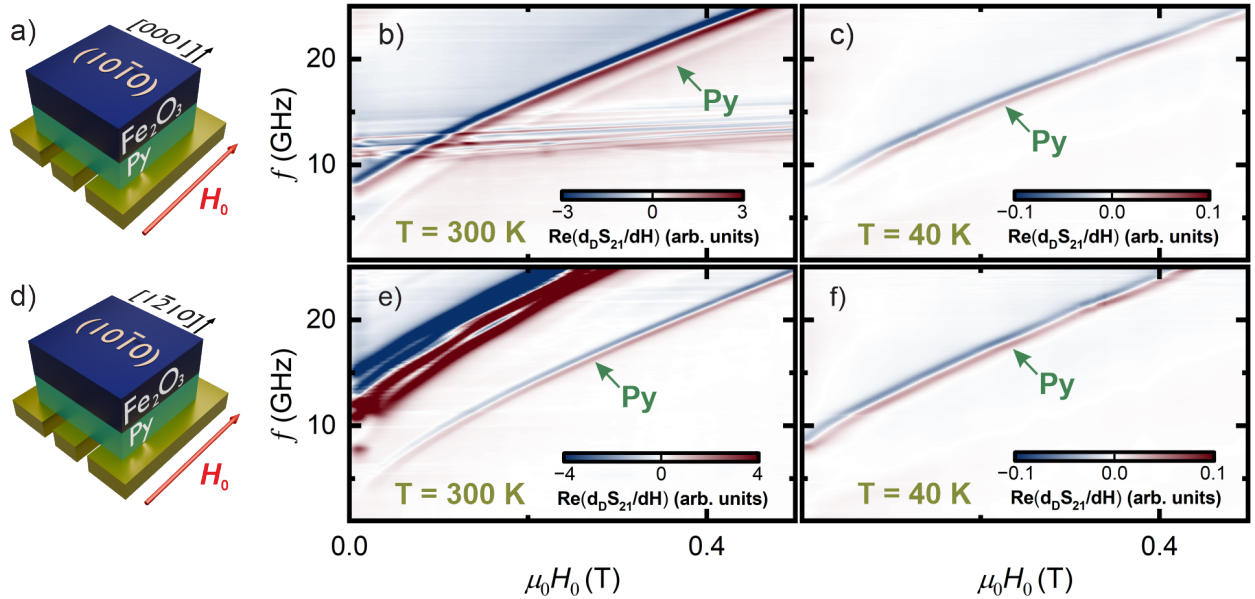

FIG. S4. FMR spectra of the  $(10\bar{1}0)$  sample measured with the external magnetic field aligned first along  $[0001]$  and then along the  $[1\bar{2}10]$  crystallographic orientation.

When the external magnetic field is aligned along the  $[1\bar{2}10]$  direction (Fig.S4),  $\alpha\text{-Fe}_2\text{O}_3$  exhibits a set of resonance frequencies ranging from 10 to 13 GHz at zero field (Fig.S4 (b)). All these resonance frequencies increase as the strength of  $H_0$  increases. In this configuration, the Py signal shows a modest enhancement, reaching up to 3 GHz at zero external field.

At 40 K, the sample exhibits a clear enhancement in the Py signal when the external field is zero, with resonance frequencies reaching up to 8 GHz. This observation indicates the presence of exchange coupling at the interface. Notably, at this low temperature, the strength of the interfacial exchange coupling depends on the magnitude of the applied external magnetic field.

At high  $H_0$ , the sample demonstrates orientation-dependent behavior with respect to the applied crystallographic field direction. As  $H_0 \parallel [0001]$ , the Py signal remains unaffected by a decrease in temperature, even at large field values. Conversely, for  $H_0 \parallel [1\bar{2}10]$ , the Py signal exhibits a noticeable enhancement as the temperature decreases, even under high  $H_0$ .

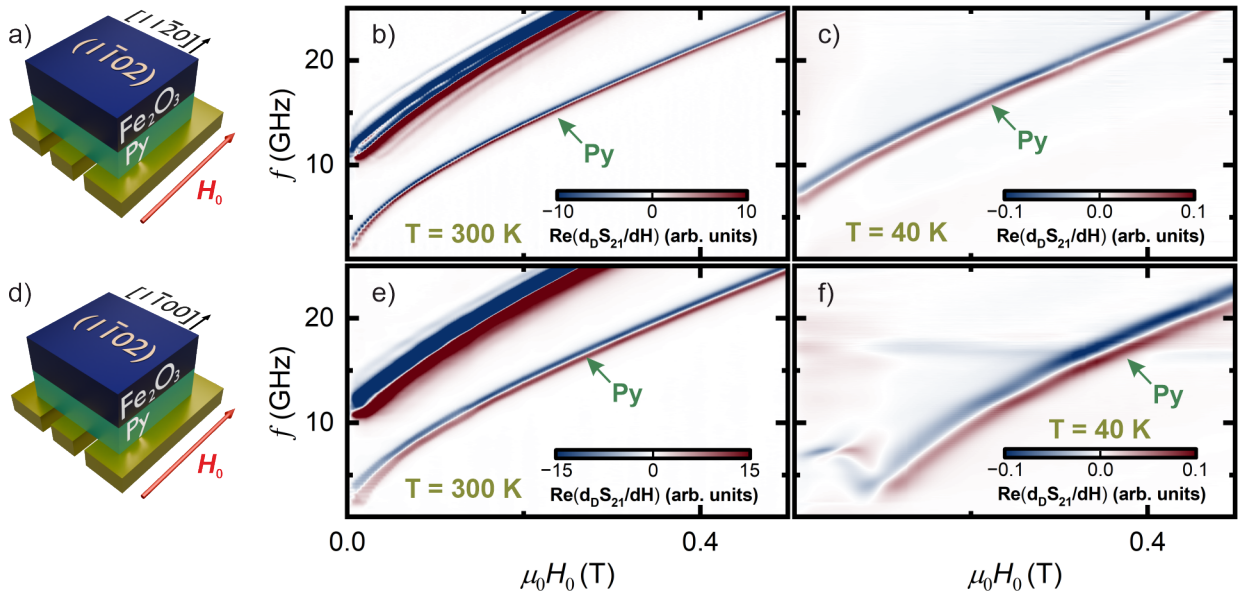

FIG. S5.  $(1\bar{1}02)$  sample, (a) measured along  $[1\bar{1}20]$ , and (d) along a projection of  $[1\bar{1}00]$  crystal orientation.

Finally, the FMR spectra for the  $(1\bar{1}02)$  sample were measured, as illustrated in Fig. S5. Initially, the external magnetic field was applied along the  $[1\bar{1}20]$  in-plane orientation (Fig. S5(a)). At 300 K, a modest enhancement of the Py signal is observed up to 2.5 GHz. This enhancement becomes more pronounced as the temperature decreases, with the Py

signal extending up to 7 GHz at zero external field. When the external field is aligned along a projection onto the  $[1\bar{1}00]$  crystal orientation, similar behavior is observed at higher temperatures. At lower temperatures, interfacial exchange coupling is evident, as indicated by an enhancement of the Py signal up to 6.5 GHz at zero field. When the external field is increased to 0.07 T, a significant increase in the Py signal is observed, suggesting a decoupling of the spin systems of the layers at the interface, resulting in the absence of interfacial exchange coupling. Beyond this field strength, the Py signal follows the Kittel uniform mode.

For this sample, in both in-plane orientations of the external magnetic field, the Néel vector projects onto the magnetization vector below  $T_M$ . This is due to the  $33^\circ$  angle between the  $[1\bar{1}02]$  direction and the c-axis. According to our model, the enhancement in the Py signal at low temperatures can be understood by the fact that the magnetization vector and the projection of the Néel vector are parallel to each other, resulting in coupling of the layers at the interface (see Fig. S7 (c) and (d)).

### Magnetic Energy Density and Boundary Conditions

In this section we set up a phenomenological model to describe the coupled ground state of  $\alpha\text{-Fe}_2\text{O}_3/\text{Py}$ . We use the magnetic anisotropy energy density of  $\alpha\text{-Fe}_2\text{O}_3$  in the easy-axis phase [6]

$$w_{\text{ani}} = 2 M_S \left( \frac{1}{2} H_{\text{ex}} \vec{m}^2 - \frac{1}{2} H_{2\parallel} n_z^2 + H_{\text{DMI}} (m_x n_y - m_y n_x) - \vec{H} \cdot \vec{m} \right), \quad (1)$$

where  $M_S$  is the sublattice magnetization,  $H_{\text{ex}}$  is the exchange field which keeps the magnetic sublattices antiparallel,  $H_{\text{DMI}} > 0$  is the homogeneous *DMI* field responsible for a small canting and thus a small magnetization in the easy-plane phase,  $H_{2\parallel} > 0$  is the uniaxial anisotropy field below the Morin transition and  $\vec{H} = \mu_0 \vec{H}_0$  is the applied magnetic field. Static states are obtained from the minimization of the above energy expression with respect to the magnetic variables  $\vec{m}$  (net magnetization) and  $\vec{n}$  (Néel vector), which in general are related due to the normalization conditions far below the *Néel* temperature

$$\vec{m} \cdot \vec{n} = 0, \quad \vec{m}^2 + \vec{n}^2 = 1. \quad (2)$$

Assuming that the magnetization is small and minimizing the energy with respect to the magnetization, we obtain

$$\vec{m} = \frac{1}{H_{\text{ex}}} \left( \vec{n} \times \vec{H} \times \vec{n} + \vec{H}_{\text{DMI}} \times \vec{n} \right). \quad (3)$$

We insert this expression into Eqn. (1) and rescale the anisotropy constant  $\bar{H}_{2\parallel} = H_{2\parallel} - H_{\text{DMI}}^2/H_{\text{ex}}$ . The magnetic ground state of the AFM is given through the competition between the internal easy-axis  $\bar{H}_{2\parallel}$ , the field-induced anisotropy  $H^2/H_{\text{ex}}$  and a unidirectional anisotropy that results from the combined effect of DMI and the external magnetic field.

In order to obtain the general case, we add an in-plane anisotropy and arrive at the full magnetic anisotropy energy density for  $\alpha\text{-Fe}_2\text{O}_3$  in Eqn. (4) [6], Permalloy in Eqn. (5) and the *surface* energy density of the interface exchange coupling in Eqn. (6). Our parameters are listed in Tab. S1.

TABLE S1. Material parameters for  $\alpha$ -Fe<sub>2</sub>O<sub>3</sub>.

|                        |                                    |            |
|------------------------|------------------------------------|------------|
| $T_M$                  | 260 K                              | [3, 4]     |
| $T_N$                  | 950 K                              | [2]        |
| $\gamma$               | 0.0001                             | [7]        |
| $a$                    | 5.067 Å                            | [1]        |
| $c$                    | 13.882 Å                           | [1]        |
| $M_S$                  | $4.23 \mu_B = 3.31 \cdot 10^6$ A/m | [8]        |
| $\bar{H}_{2\parallel}$ | $\pm 24$ mT                        | [9]        |
| $H_{\text{ex}}$        | 1040 T                             | [10]       |
| $H_{\text{DMI}}$       | 2.75 T                             | [9]        |
| $H_{\text{6an}}$       | 137 $\mu$ T                        | [9]        |
| $f$                    | 0.19 THz – 0.5 THz                 | [11]       |
| $A_F$                  | $4.4 \text{ pJ m}^{-1}$            | Int. Comm. |
| $M_F$                  | $8.6 \times 10^5 \text{ A m}^{-1}$ | [12]       |

$$w_{\text{AF}} = M_S \left( -\frac{1}{2} \bar{H}_{2\parallel}(\text{T}) n_z^2 - \frac{H_{\text{DMI}}}{H_{\text{ex}}} \vec{n} \cdot (\vec{H} \times \hat{z}) + \frac{(\vec{n} \cdot \vec{H})^2}{2 H_{\text{ex}}} \right) - \frac{1}{6} M_S H_6 (n_x^2 - n_y^2) (4(n_x^2 - n_y^2)^2 - 3), \quad (4)$$

$$w_F = \frac{1}{2} \mu_0 M_F^2 (\hat{m}_F \cdot \hat{e})^2 - M_F \hat{m}_F \cdot \vec{H}, \quad (5)$$

$$w_{\text{int}} = -J_{\text{int}} \xi M_S M_F \delta(\hat{e} \cdot \vec{r}) \hat{m}_F \cdot \hat{n}, \quad (6)$$

where we renormalized the AFM saturation sublattice magnetization to the total saturation magnetization,  $H_{\text{DMI}} > 0$  is the homogeneous DMI field that leads to a small spin canting and finite magnetization in the easy-plane phase,  $H_{\text{6an}} > 0$  is the in-plane anisotropy resulting from the rhombohedral symmetry of  $\alpha$ -Fe<sub>2</sub>O<sub>3</sub>. The out-of-plane anisotropy  $\bar{H}_{2\parallel}(\text{T})$  is temperature dependent, such that it is positive below the Morin temperature and changes sign at the Morin transition. The normal vector of the sample's surface is given by  $\hat{e}$  (which in our case is  $\hat{z}$ ) and  $\vec{r}$  is the location vector. The ground state of the FM magnetization  $\vec{m}_F$  is characterized by the demagnetization term that forces the FM magnetization into the sample plane ( $\mu_0$  is the vacuum permeability). The FM magnetization couples to an external

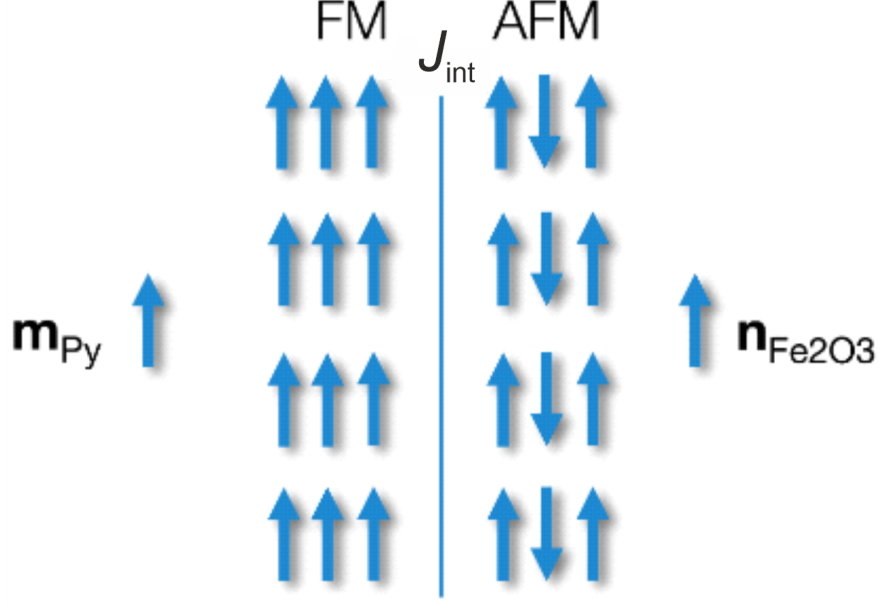

FIG. S6. Parallel Coupling of the AFM Néel vector and the FM magnetization. We assume a layered sublattice structure of  $\alpha$ -Fe<sub>2</sub>O<sub>3</sub> at the surface. Thus, we can model the interface exchange coupling as the direction interaction that favors parallel alignment of the AFM Néel vector and the FM magnetization.

field via the Zeeman term with an external field  $\vec{H} = \mu_0 \vec{H}_0$ . We model the interface exchange coupling as a direct coupling between the *Néel* vector and the FM magnetization, mediated by the coupling strength  $J_{\text{int}}$  and the infinitesimal length scale  $\xi$ , as schematically indicated in Fig. S6. The FM magnetization vector is  $\vec{m}_F = M_F \hat{m}_F = M_F (m_{F,x}, m_{F,y}, m_{F,z})^T$  and the AFM Néel vector is  $\vec{n} = M_S \hat{n} = M_S (n_x, n_y, n_z)^T$ .

In the general case we parametrize the *Néel* vector and the magnetization in spherical coordinates

$$\hat{n} = (\sin \theta_A \cos \phi_A, \sin \theta_A \sin \phi_A, \cos \theta_A)^T, \quad (7)$$

$$\hat{m}_F = (\sin \theta_F \cos \phi_F, \sin \theta_F \sin \phi_F, \cos \theta_F)^T. \quad (8)$$

### *Antiferromagnetic Ground States*

Before considering the impact of interface exchange coupling on the magnetic state of  $\alpha\text{-Fe}_2\text{O}_3$ , we want to study its isolated magnetic ground state. In the absence of a magnetic field, the energy density Eqn. (4) simplifies to

$$U_{\text{AF}} = -H_{\text{ex}} \bar{H}_{2\parallel}(\text{T}) \cos^2 \theta_A - \frac{1}{3} H_{\text{ex}} H_{6\text{an}} \sin^6 \theta_A \cos(6\phi_A), \quad (9)$$

$$(10)$$

where the potential energy was introduced by  $U_{\text{AF}} = 2H_{\text{ex}} / M_S \cdot w_{\text{AF}}$ .

We directly detect that the ground state emerges from the competition of the uniaxial and the in-plane anisotropy. The uniaxial anisotropy  $\bar{H}_{2\parallel}(\text{T})$  is the dominant one  $|\bar{H}_{2\parallel}| > H_{6\text{an}}$  and changes sign at the Morin transition point at  $\sim 260$  K from positive to negative. Hence, the Néel vector in the low temperature phase prefers to point along the z-direction, while an easy plane orientation is preferred in the high temperature phase. Additionally, the sixth order in-plane anisotropy  $H_{6\text{an}}$  determines the six easy axis direction in the xy-plane for  $\phi_A = n \cdot \pi/3$  with  $n = 0, \dots, 5$ .

#### Magnetic Field along the Easy Axis:

Owing to the DMI, an applied magnetic field alters the magnetic ground state significantly. First we will consider an applied magnetic field along the easy axis. Thus, DMI plays no role. For simplicity we neglect the in-plane anisotropy

$$U_{\text{AF}} = \left( -H_{\text{ex}} \bar{H}_{2\parallel}(\text{T}) + H_z^2 \right) \cos^2 \theta_A, \quad (11)$$

In the low temperature phase we find a spin-flop transition for  $H > H_{\text{sf}} := \sqrt{H_{\text{ex}} \bar{H}_{2\parallel}}$ , where the Néel vector flips from  $\vec{n} \parallel \hat{z}$  into  $\vec{n} \perp \hat{z}$ . When we include the in-plane anisotropy, the degeneracy of the direction of the Néel vector in the xy-plane is lifted and the spin-flop field is modified to  $H_{\text{sf}} := \sqrt{H_{\text{ex}} (\bar{H}_{2\parallel} + H_{6\text{an}})}$ . In this case the reorientation of the Néel vector is not an instantaneous flip any more, but a very quick, smooth reorientation. In the high temperature phase, the Néel vector is always in the xy-plane and the in-plane anisotropy governs its direction.

### Magnetic Field perpendicular to the Easy Axis:

Without the in-plane anisotropy the Néel vector directions in the xy-plane are degenerate, Thus, an in-plane magnetic field will have equivalent effects on the Néel vector regardless of its direction. We choose  $\vec{H} \parallel \hat{y}$ , which gives

$$\begin{aligned}
U_{\text{AF}} = & - H_{\text{ex}} \bar{H}_{2\parallel}(\text{T}) \cos^2 \theta_A \\
& + H_y^2 \sin^2 \theta_A \sin^2 \phi_A \\
& - 2 H_{\text{DMI}} H_y \sin \theta_A \cos \phi_A,
\end{aligned} \tag{12}$$

$\vec{H} \parallel \hat{y}$  means that  $\vec{n}$  rotates in the xz-plane, such that we can parametrize the Néel vector by  $n_x = \sin \theta$ ,  $n_z = \cos \theta$ . It follows that below the spin-flop field  $|\vec{H}| < H_{\text{DMIsf}} := H_{\text{sf}}^2/H_{\text{DMI}}$  the solution is  $n_x = H/H_{\text{DMIsf}}$  and  $n_z = \pm \sqrt{1 - n_x^2}$ . States with opposite sign of  $n_z$  have the same energy, while the sign of  $n_x$  depends on the direction of the applied field. Thus, domains with opposite directions will rotate in opposite directions towards the x-axis. Above the spin-flop transition  $|H| > H_{\text{DMIsf}}$   $n_z = 0$  and  $n_x = \pm 1$  depending on the direction of the field. The in-plane anisotropy induces a small perturbation to the above results, giving preference to a canting towards the nearest in-plane easy axis and also modifying the spin-flop fields.

In summary, we found that for low temperatures the magnetic ground state is in the easy-axis phase, where the Néel vector aligns with the z-axis. A magnetic field applied along the easy axis can induce a spin-flop transition into the easy-plane, where the in-plane anisotropy governs the preferred directions. Moreover, in the spin flop phase the sublattices fall out of alignment to form a non-zero magnetization. If the magnetic field is applied in the easy plane, the Néel vector smoothly rotates away from the easy axis and into a direction orthogonal to the magnetic field is induced due to DMI. Here, again the in-plane anisotropy gives additional constraints through the in-plane easy axes. In the high-temperature regime above the Morin temperature the Néel vector is in the plane in its canted phase. Its orientation is then given by the superposition of alignment with the in-plane easy axes and a rotation orthogonal to the applied field.

## Numerical Solution of the Ferromagnetic Resonance Spectrum

We calculate the FM resonance spectrum of Permalloy, that is interface exchange coupled to  $\alpha\text{-Fe}_2\text{O}_3$ , in a three-step procedure. First, we solve the AFM equation of state and obtain the AFM magnetic ground state. In this step, we only consider the AFM  $\alpha\text{-Fe}_2\text{O}_3$  layer. That means the effect of interface exchange coupling is not included, but for instance the influences of an external field and DMI acting on the Néel vector are considered. We justify this approximation with the relative contribution of the interactions on the energy of the system.

In the second step, we determine the FM ground state magnetization orientation, taking into account interface exchange coupling of the FM magnetization to the previously determined AFM Néel vector. We now have obtained the ground state orientations of both the AFM Néel vector and the FM magnetization, as shown in Fig. S7.

In the third and final step we consider a perturbation on top of the FM ground state and calculate the magnon spectrum.

In order to find the magnetic ground state for arbitrary field directions and using the full anisotropy of  $\alpha\text{-Fe}_2\text{O}_3$ , we use a numerical approach to solve the equations of state for the Néel vector parametrization angles  $\theta_A$  and  $\phi_A$  and the FM magnetization angles  $\theta_F$  and  $\phi_F$  in spherical coordinates

$$\gamma \dot{\theta}_{\text{AF}} + \frac{\partial w_{\text{AF}}}{\partial \theta_{\text{AF}}} = 0, \quad (13)$$

$$\gamma \dot{\phi}_{\text{AF}} + \frac{\partial w_{\text{AF}}}{\partial \phi_{\text{AF}}} = 0, \quad (14)$$

$$\gamma \dot{\theta}_F + \frac{\partial(w_F + w_{\text{int}}/d_F)}{\partial \theta_F} = 0, \quad (15)$$

$$\gamma \dot{\phi}_F + \frac{\partial(w_F + w_{\text{int}}/d_F)}{\partial \phi_F} = 0, \quad (16)$$

where  $\gamma$  governs the numerical rate of relaxation into the minimum energy state,  $d_F$  is the FM layer thickness and  $\dot{\phantom{x}}$  signifies a simulation step. The equilibrium angle  $\varphi_0$  is the angle between the FM magnetization and the AFM Néel vector in their respective ground state.

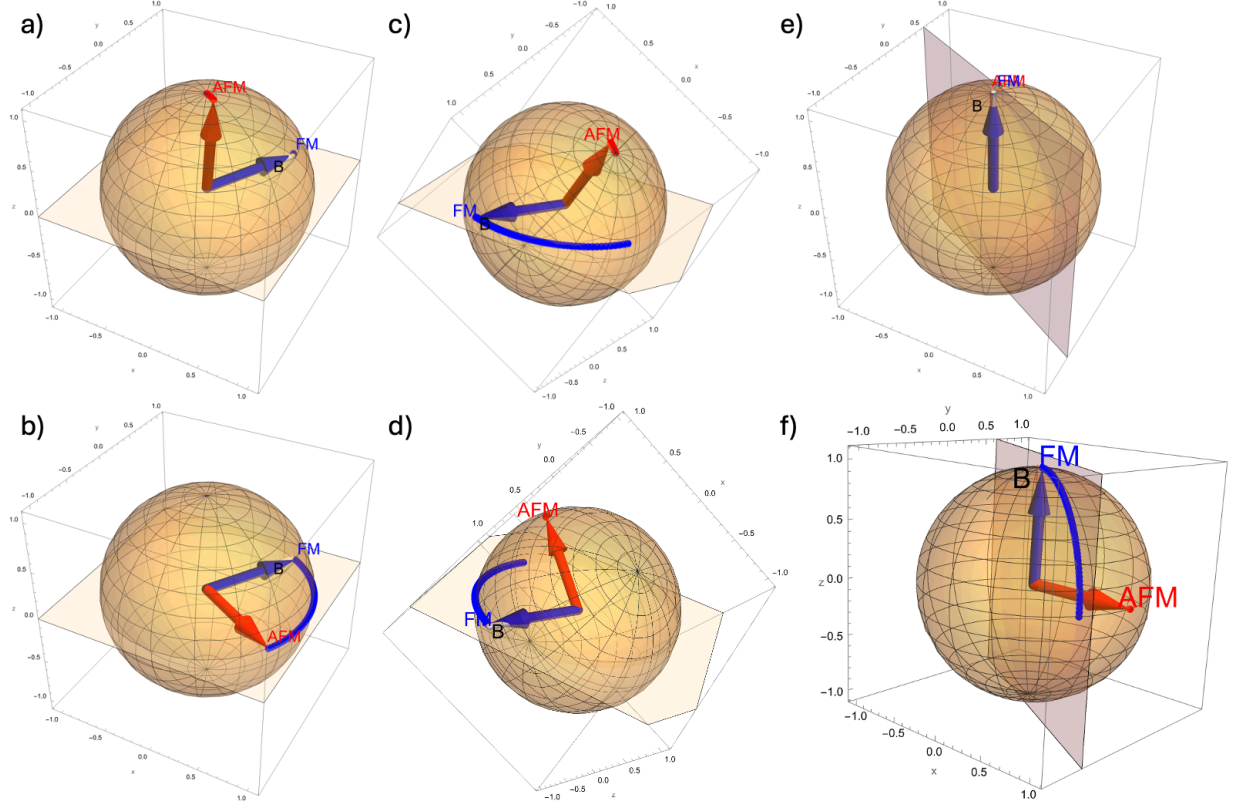

FIG. S7. Equilibrium orientation of the coupled FM magnetization (blue arrow) and AFM Néel vectors (red arrow). Also shown is the external magnetic field  $\vec{B}$  direction. The upper row a), c), e) shows the orientations for the easy axis phase ( $T < T_M$ ), while the lower row b), d), f) shows the easy plane phase ( $T > T_M$ ). Rotation of the FM magnetization and the AFM Néel vector due to interface exchange coupling is indicated by colored lines on the unit sphere. The first column a), b) shows the c-cut system, the second column c), d) the r-cut system and the third column e), f) the a-cut system.

### *Ferromagnetic Resonance*

After we have calculated and fixed the Néel vector orientation in  $\alpha\text{-Fe}_2\text{O}_3$ , we determine the influence of the AFM state and especially the interface exchange coupling on the FMR resonance using the FM Lagrangian

$$\mathcal{L} = \frac{M_F}{\gamma} (1 - \cos\theta) \dot{\phi} - w(\theta, \phi) - M_F \hat{m}_F \vec{h}, \quad (17)$$

where the magnetization is parametrized in spherical coordinates with the angles  $\theta = \theta_F$

and  $\phi = \phi_F$ ,  $w = w_F + w_{\text{int}}/d_F$  and  $\vec{h} = h_{\text{amp}} \vec{h}_{\text{ac}} \cdot e^{i\omega t}$  is the FMR oscillating field. The corresponding *Euler-Lagrange* equations are

$$0 = -\frac{\partial w}{\partial \theta} + \frac{M_F}{\gamma} \sin \theta \dot{\phi} - M_F h_{\text{amp}} e^{i\omega t} (h_{\text{ac},x} \cos \theta \cos \phi + h_{\text{ac},y} \cos \theta \sin \phi - h_{\text{ac},z} \sin \theta), \quad (18)$$

$$0 = \frac{M_F}{\gamma} \sin \theta \dot{\theta} + \frac{\partial w}{\partial \theta} + M_F h_{\text{amp}} e^{i\omega t} (-h_{\text{ac},x} \sin \theta \sin \phi + h_{\text{ac},y} \sin \theta \cos \phi). \quad (19)$$

Now we expand around the equilibrium solution  $\theta_0, \phi_0$  determined as shown above

$$\theta = \theta_0 + \delta \theta, \quad (20)$$

$$\phi = \phi_0 + \delta \phi. \quad (21)$$

We only consider terms linear in  $\delta \phi, \delta \theta, h_{\text{amp}}$ . When performing the *Taylor* expansion, the components of the *Hesse* matrix of the energy density appear. The components are in the original basis and not diagonalized.

$$0 = -\delta \dot{\phi} + \frac{\gamma}{M_F} \sin^{-1} \theta_0 \frac{\partial^2 w}{\partial \theta^2} \Big|_{\theta_0, \phi_0} \delta \theta + \frac{\gamma}{M_F} \sin^{-1} \theta_0 \frac{\partial^2 w}{\partial \theta \partial \phi} \Big|_{\theta_0, \phi_0} \delta \phi - \gamma \sin^{-1} \theta_0 h_{\text{amp}} e^{i\omega t} (h_{\text{ac},x} \cos \theta_0 \cos \phi_0 + h_{\text{ac},y} \cos \theta_0 \sin \phi_0 - h_{\text{ac},z} \sin \theta_0) \quad (22)$$

$$0 = \delta \dot{\theta} + \frac{\gamma}{M_F} \sin^{-1} \theta_0 \frac{\partial^2 w}{\partial \phi \partial \theta} \Big|_{\theta_0, \phi_0} \delta \theta + \frac{\gamma}{M_F} \sin^{-1} \theta_0 \frac{\partial^2 w}{\partial \phi^2} \Big|_{\theta_0, \phi_0} \delta \phi + \gamma \sin^{-1} \theta_0 h_{\text{amp}} e^{i\omega t} (-h_{\text{ac},x} \sin \theta_0 \sin \phi_0 + h_{\text{ac},y} \sin \theta_0 \cos \phi_0). \quad (23)$$

We simplify

$$0 = -\delta \dot{\phi} + A_{\theta\theta} \delta \theta + A_{\theta\phi} \delta \phi - H_\theta(t), \quad (24)$$

$$0 = \delta \dot{\theta} + A_{\phi\theta} \delta \theta + A_{\phi\phi} \delta \phi + H_\phi(t), \quad (25)$$

where the components of the *Hesse* matrix of the FM energy density are

$$A_{\theta\theta} = \frac{\gamma}{M_F} \sin^{-1}\theta_0 \frac{\partial^2 w}{\partial \theta^2} \big|_{\theta_0, \phi_0}, \quad (26)$$

$$A_{\phi\theta} = A_{\theta\phi} = \frac{\gamma}{M_F} \sin^{-1}\theta_0 \frac{\partial^2 w}{\partial \theta \partial \phi} \big|_{\theta_0, \phi_0}, \quad (27)$$

$$A_{\phi\phi} = \frac{\gamma}{M_F} \sin^{-1}\theta_0 \frac{\partial^2 w}{\partial \phi^2} \big|_{\theta_0, \phi_0}. \quad (28)$$

We parametrize the perturbation as

$$\delta\theta = \bar{\theta} e^{i\omega t}, \quad (29)$$

$$\delta\phi = \bar{\phi} e^{i\omega t}. \quad (30)$$

Thus, our equations of motion become

$$0 = -i\omega\bar{\phi} + A_{\theta\theta}\bar{\theta} + A_{\theta\phi}\bar{\phi} - H'_\theta(t), \quad (31)$$

$$0 = i\omega\bar{\theta} + A_{\phi\theta}\bar{\theta} + A_{\phi\phi}\bar{\phi} + H'_\phi(t), \quad (32)$$

where  $H'_\theta(t)$ ,  $H'_\phi(t)$  do not contain the exponentials anymore. We can solve

$$\bar{\theta} = \frac{(i\omega - A_{\theta\phi})\bar{\phi} + H_\theta}{A_{\theta\theta}}, \quad (33)$$

and reinserting into Eqn. (32) yields

$$(i\omega + A_{\phi\theta})(i\omega - A_{\phi\theta})\bar{\phi} + (i\omega + A_{\phi\theta})H_\theta + A_{\phi\phi}A_{\theta\theta}\bar{\phi} + H_\phi A_{\theta\theta} = 0, \quad (34)$$

from which we find the resonance condition

$$(i\omega + A_{\phi\theta})(i\omega - A_{\phi\theta}) + A_{\phi\phi}A_{\theta\theta} = 0, \quad (35)$$

and the resonance frequency

$$\omega = \sqrt{A_{\phi\phi}A_{\theta\theta} - A_{\phi\theta}^2}. \quad (36)$$

We have now obtained the equilibrium orientation of the AFM Néel vector and the FM magnetization. Furthermore, we have derived the FM magnon spectrum in presence of interface exchange coupling to the AFM Néel vector. We do not consider the back-action of the FM magnetization on the AFM Néel vector.

|                | $T < T_M, H_{\parallel}$ | $T < T_M, H_{\perp}$ |
|----------------|--------------------------|----------------------|
| c-cut          | parallel to              | perpendicular to     |
| (0001)         | $[11\bar{2}0]$           | $[11\bar{2}0]$       |
| a-cut          | parallel to              | perpendicular to     |
| $(11\bar{2}0)$ | $[0001]$                 | $[0001]$             |
| e-cut          | parallel to              | perpendicular to     |
| $(10\bar{1}0)$ | $[0001]$                 | $[0001]$             |
| r-cut          | parallel to              | perpendicular to     |
| $(1\bar{1}02)$ | $[11\bar{2}0]$           | $[11\bar{2}0]$       |

TABLE S2. Experimental measurements of the FMR spectrum of coupled Permalloy were performed for these crystal cuts of the  $\alpha$ -Fe<sub>2</sub>O<sub>3</sub> layer surface. All samples were measured for two applied field directions, as indicated. The measurements were repeated for temperatures both above and below Morin temperature.

### Fitting of Experimental Data

$\alpha$ -Fe<sub>2</sub>O<sub>3</sub> has a hexagonal crystal structure. The samples that were used in this work were identified using hexagonal *Miller-Bravais* indices. The hexagonal coordinate system exhibits rotational invariance for  $\alpha = 120^\circ$  in its basal plane. We can thus describe the system using a basis constituent of four vectors:  $\vec{a}_1, \vec{a}_2, \vec{a}_3$  are in the basal plane at an angle of  $120^\circ$  to each other, and  $\vec{c}$  points out-of-plane. This coordinate system is overdetermined by  $\vec{a}_3 = -(\vec{a}_1 + \vec{a}_2)$ . Our theoretical model uses the cartesian coordinate system, where  $\vec{x}$  is parallel to  $\vec{a}_1$  and  $\vec{z}$  is parallel to  $\vec{c}$  [13, 14].

FMR spectra were experimentally obtained for a range of temperatures both above and below Morin transition. We repeat our measurements for two orthogonal applied field directions for  $\alpha$ -Fe<sub>2</sub>O<sub>3</sub> samples, where the Permalloy layer has been applied to the c-, a-, e- and r-cut surfaces, as indicated in Tab. S2. We show the crystal cut surfaces in Fig. S2.

We fit the experimentally obtained data and use our theoretical modeling to extract the interface exchange coupling strength from the zero field frequency gap of the Permalloy

signal. Using the value from this estimation we can numerically replicate the experimentally observed spectrum and determine the FM magnetization's and AFM Néel vector's ground state orientation in presence of interface exchange coupling. Specifically, we can also discern the cases in which interface exchange coupling leads to coupled dynamics, and cases where it does not.

Our key result is, that strong interface exchange coupling occurs, if the FM magnetization and a sufficiently large projection of the AFM Néel vector both lie in the sample's surface plane. This deciding relative orientation can be influenced by temperature (which changes the Néel vector of  $\alpha$ -Fe<sub>2</sub>O<sub>3</sub> ground state orientation), crystal cut (which adjusts the relative orientation of the AFM Néel vector and the FM magnetization) and applied field (which affects the orientation of the FM magnetization most strongly).

---

\* E-Mail: h.alhamdo@rptu.de; These authors contributed equally.

† These authors contributed equally.

- [1] Rohrbach, A., Hafner, J. & Kresse, G. Ab initio study of the (0001) surfaces of hematite and chromia: Influence of strong electronic correlations. *Phys. Rev. B* **70**, 125426 (2004).
- [2] Morrish, A. H. *Canted Antiferromagnetism: Hematite* (World Scientific, 1995).
- [3] Chou, S. G. *et al.* High-resolution terahertz optical absorption study of the antiferromagnetic resonance transition in hematite ( $\alpha$ -Fe<sub>2</sub>O<sub>3</sub>). *J. Phys. Chem. C* **116**, 16161–16166 (2012).
- [4] Morin, F. Magnetic susceptibility of  $\alpha$ -Fe<sub>2</sub>O<sub>3</sub> and  $\alpha$ -Fe<sub>2</sub>O<sub>3</sub> with added titanium. *Phys. Rev.* **78**, 819 (1950).
- [5] Maier-Flaig, H. *et al.* Note: Derivative divide, a method for the analysis of broadband ferromagnetic resonance in the frequency domain. *Rev. Sci. Instrum.* **89**, 076101 (2018).
- [6] Lebrun, R. *et al.* Long-distance spin-transport across the Morin phase transition up to room temperature in ultra-low damping single crystals of the antiferromagnet  $\alpha$ -Fe<sub>2</sub>O<sub>3</sub>. *Nat. Commun.* **11**, 6332 (2020).
- [7] Danneegger, T. *et al.* Magnetic properties of hematite revealed by an ab initio parameterized spin model. *Phys. Rev. B* **107**, 184426 (2023).
- [8] Hill, A. H. *et al.* Neutron Diffraction Study of Mesoporous and Bulk Hematite,  $\alpha$ -Fe<sub>2</sub>O<sub>3</sub>. *Chem. Mater.* **20**, 4891–4899 (2008).
- [9] Lebrun, R. *et al.* Anisotropies and magnetic phase transitions in insulating antiferromagnets determined by a Spin-Hall magnetoresistance probe. *Commun. Phys.* **2**, 50 (2019).
- [10] Besser, P. J., Morrish, A. H. & Searle, C. W. Magnetocrystalline Anisotropy of Pure and Doped Hematite. *Phys. Rev.* **153**, 632–640 (1967).
- [11] Białek, M., Zhang, J., Yu, H. & Ansermet, J.-P. Antiferromagnetic resonance in  $\alpha$ -Fe<sub>2</sub>O<sub>3</sub> up to its Néel temperature. *Appl. Phys. Lett.* **121** (2022).
- [12] Nahrwold, G. *et al.* Structural, magnetic, and transport properties of Permalloy for spintronic experiments. *J. Appl. Phys.* **108** (2010).
- [13] Fabian, K., Robinson, P., Mcenroe, S. A., Heidelbach, F. & Hirt, A. M. *The Earth’s Magnetic Interior* (Springer Netherlands, Dordrecht, 2011).
- [14] Kraushofer, F. *et al.* Atomic-Scale Structure of the Hematite  $\alpha$ -Fe<sub>2</sub>O<sub>3</sub> (1 $\bar{1}$ 02) “R-Cut” Surface.

*J. Phys. Chem. C* **122**, 1657–1669 (2018).
